# Supplementary material for: Determination of spin relaxation times in heavy metals via 2nd harmonic spin injection magnetoresistance
Source: arXiv:1705.03149 source file (2017-05-09)
Supplement: Supplementary file 1 [file Supplementary_Information.pdf]

# Supplementary Information

## Determination of spin relaxation times in heavy metals via 2nd harmonic spin injection magnetoresistance

C. Fang[1], C. H. Wan[1], X. M. Liu[3], B. S. Yang[1], J. Y. Qin[1], B. S. Tao[1], H. Wu[1], X. Zhang[1], Z. M. Jin[3], A. Hoffmann[2], X. F. Han[1]

1. Institute of Physics, Chinese Academy of Sciences, Beijing, 100190, China

And University of Chinese Academy of Sciences, Beijing 100049, China.

2. Materials Science Division, Argonne National Laboratory, 9700 S. Cass Avenue, Lemont, IL 60439.

3. Department of Physics, Shanghai University, Shanghai 200444, China.

## A. TEM characterization of the cross section of thin films

Transmission Electron Microscope (TEM) pattern of Ta/MgO/CoFeB and Pt/MgO/CoFeB in Figure R1 shows that the thickness of MgO layer is not very uniform. The yellow arrows in Figure R1 points out the area where the thickness is less than surrounding area and could probably act as the inhomogeneous area which leads to a larger tunneling rate and may account for a reduction of the effective tunneling area.

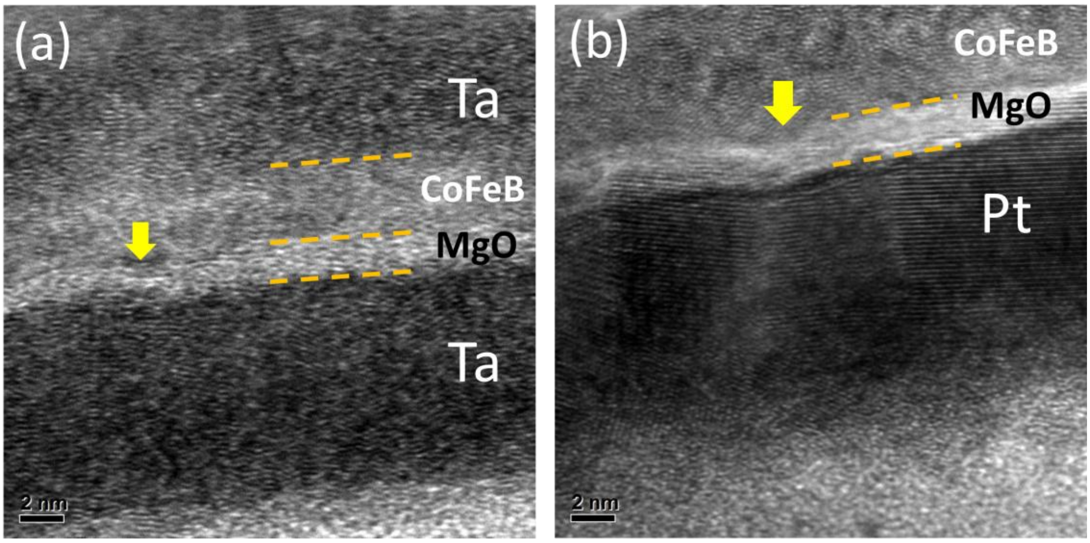


Figure S1 TEM pattern of (a) Ta/MgO/CoFeB and (b) Pt/MgO/CoFeB. Yellow arrows in the patterns point to the inhomogeneous area of the MgO barrier.

## B. Data of second harmonic measurement

The mean value and deviation in Fig. 4 in the letter are acquired by investigating the same device for many times. We have also performed the same experiments on four more Ta devices and three more Pt devices and acquired the deviation among the different samples as shown in Figure S2 and Figure S3. The devices of the same type stacks are fabricated at the same time on one chip. The spin relaxation time in Ta is (13.1±0.6) ps at 10 K and decays to (7.8±1.6) ps at 300 K. Also the $\tau_{\mathrm{Pt}}$ decays from (7.3±0.6) ps to (5.0±1.6) ps as the temperature rises up.

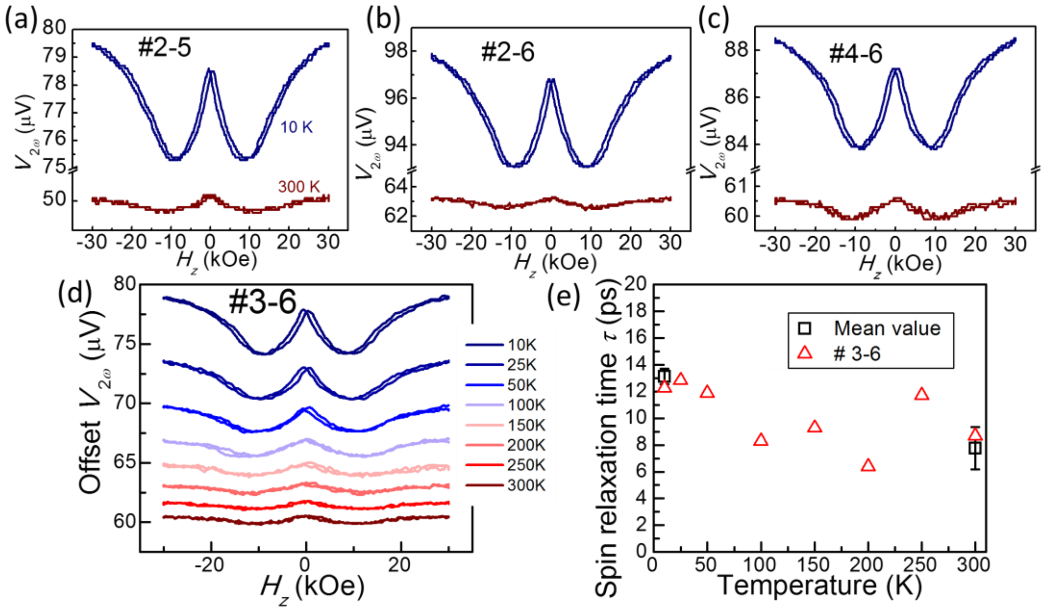


Figure S2 Second harmonic measurement data of more Ta/MgO/CoFeB devices (a)2-5, (b)2-6, (c)4-6, (d)3-6. (e) Mean spin relaxation time of different devices.

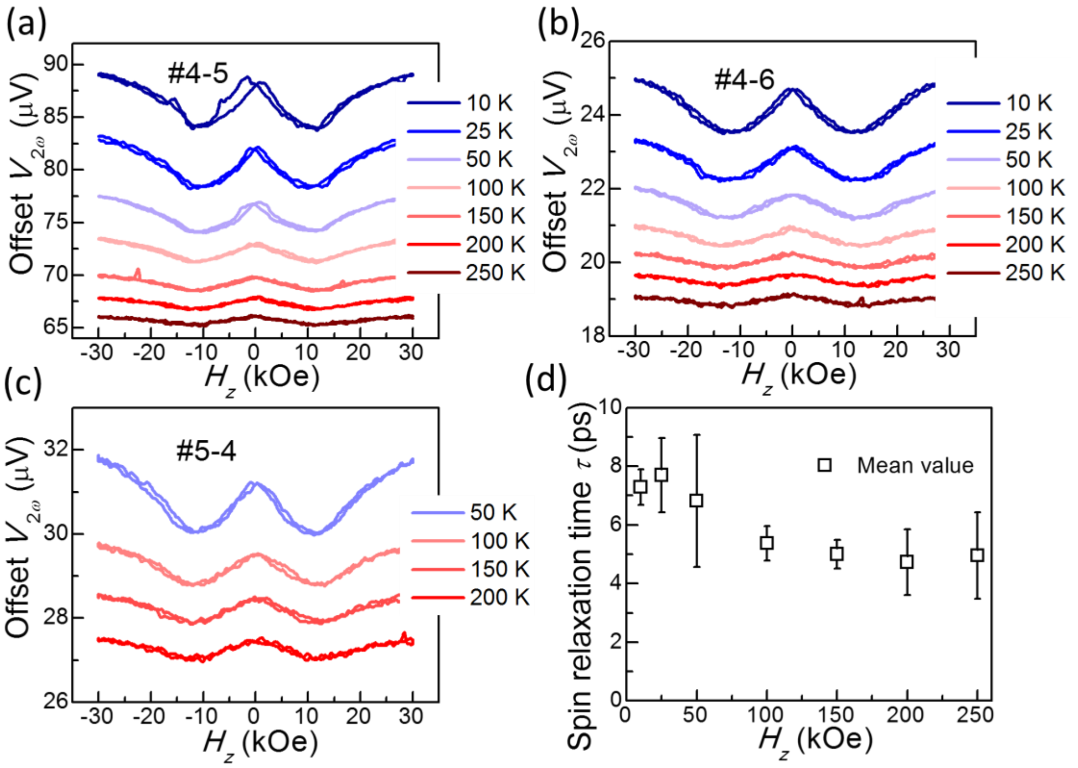


Figure S3 Second harmonic measurement data of more Pt/MgO/CoFeB devices (a) 4-5, (b) 4-6, (c) 5-4. (d) Mean spin relaxation time of different devices.

## C. Elimination of AMR effect

We adopted the patterned Ta/MgO/CoFeB and Pt/MgO/CoFeB stacks (Hall Bar Structure) with four-terminals to measure their AMR. As the first harmonic measurement data [Figure S4 (a)-(d)] shows, the variation of the resistance depending on the external magnetic field is within 5%. And the harmonic measurement appears to be not sensitive enough to acquire the AMR signal even if it exists. Furthermore, we use a DC measurement at low temperature. The DC measurement provides a clear field dependence of the resistance, which is well below the resolution of the previous first harmonic measurments. The field dependence measured in the Hall bar is not consistent with that in tunneling junctions. The MR here [Figure S4 (e) and (f)] is positive, differing from the negative one in our manuscript. Besides, we have etched the film to the bottom heavy metal layer outside the junction area and also deposited very thick Cu(80nm)/Au(20nm) electrode on top of the CoFeB/Ta/Ru films. The thick Cu/Au films shunt the majority of the current and further makes the very tiny AMR of CoFeB invisible in measuring transport properties of the junctions. Thus the AMR originating from the CoFeB is negligible and does not cause the field dependence pattern in the first and second harmonic measurement of the junctions' resistance.

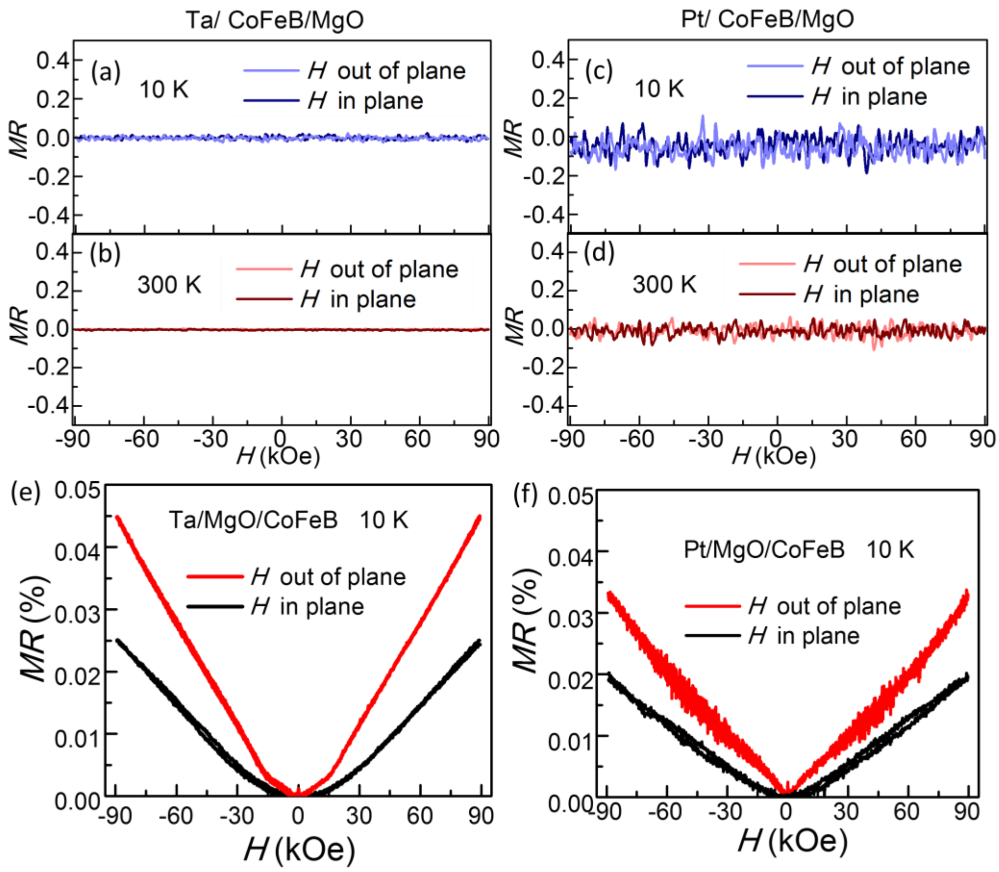


Figure S4: First harmonic AMR measurement data with patterned Ta/MgO/CoFeB stacks under (a)10K and (b)300 K, Pt/MgO/CoFeB stacks under (c)10K and (d)300 K. DC AMR measurement with (e) Ta/MgO/CoFeB and (f) Pt/MgO/CoFeB.
